# Supplementary material for: A Bilevel Optimization Scheme for Persistent Monitoring
Source: arXiv:2304.03667 source file (2023-04-07)
Supplement: Supplementary file 1 [file appendix.tex]

\section{Appendix}\label{sec:appendix}
In order to compute the exact partials of initial uncertainty $\check{R}_k$~\eqref{eq:initial:uncertainty} we must specify $\varepsilon(\psi_\ell, \varphi_{\ell+1})$. We know that the agent's trajectory from $s_k^0$ to $s_\ell^\psi$ forms a straight line of length $\Delta = \| s_\ell^\psi - s_\ell^0 \|$ with constant maximal control. Specifically, we obtain the trajectory piece $s(t) = s_\ell^0 + t \frac{s_\ell^\psi - s_\ell^0}{\Delta}$,
where we assume without loss of generality that the inner exit point is reached at time $0$ and $x_{i_k} = 0$. Using trigonometric identities, we then compute 
\begin{equation*}
    \begin{split}
        s(t)^\top s(t) 
        %&= {s_k^0}^\top s_k^0 + 2\frac{t}{\Delta} s_k^0(s_k^\psi - s_k^0) + \frac{t^2}{\Delta^2} (s_k^\psi - s_k^0)^\top (s_k^\psi - s_k^0) \\
        = \delta^2 &+ \frac{2t}{\Delta}\left(r\delta \cos\left(\psi_\ell - \psi_\ell^0\right) - \delta^2\right) \\ &+ \frac{t^2}{\Delta^2}\left(r^2 + \delta^2 - 2 r \delta \cos\left(\psi_\ell - \psi_\ell^0\right)\right),
    \end{split}
\end{equation*}
where $\psi_k$ and $\psi_k^0$ are the polar coordinate angles of the outer and inner departure points, respectively. Knowing that the uncertainty dynamics for the considered trajectory piece is nonnegative, we must compute 
\begin{equation*}
    \begin{split}
        \varepsilon &= \int_0^\Delta A - B \left(1 - \frac{s(t)^\top s(t)}{r^2}\right) dt \\
        %&= \Delta(A - B) + \frac{B}{r^2}\int_0^\Delta s(t)^\top s(t) dt \\
        &= \Delta(A - B) + \frac{\Delta B}{r^2} \left(r\delta \cos\left(\psi_\ell - \psi_\ell^0\right) - \delta^2 \right) \\ 
        &\qquad + \frac{\Delta B}{3r^2} \left( r^2 + \delta^2 - 2 r \delta \cos\left(\psi_\ell - \psi_\ell^0\right) \right)
    \end{split}
\end{equation*}
Note that $\Delta$ depends on the inner and outer departure points. The partials of $\varepsilon$ can then be computed analytically using product rule, however the precise equations are omitted here.
